# Supplementary material for: Connection between partial pressure, volatility, and the Soret effect elucidated using simulations of non-ideal supercritical fluid mixtures
Source: arXiv:2310.20005 source file (2024-05-02)
Supplement: Supplementary file 1 [file Supplementary.pdf]

# 1 Supplementary material

In this document, tabulated data is presented so that the details of the simulations could be easily replicated. Data is given in reduced units with Ar as the reference system for component 1. Moreover, data reported as Figures but not in Tables in the paper are given here in Tables S1-S8.

In Table S1, detailed simulation parameters and resulting pressure data is given for  $k_{12} = 1.35$  and  $\psi_\epsilon = 1.0$ . The same quantities are given in Table S2 for  $k_{12} = 1.35$  and  $\psi_\epsilon = 1.80$ .

Tables S3-S4 report values for  $L_1$ ,  $L_2$ , and the difference  $L_2 - L_1$  for the two simulated systems. These data points are displayed in the text in Fig. 2.

Tables S5-S6 report  $L_1^T$ ,  $L_2^T$ , and the differences  $L_2^T - L_1^T$  for the two simulated systems. These data points are displayed in the text in Figs. 2.

Tables S7-S8 report  $\gamma_1^S$ ,  $\gamma_2^S$ , and the difference  $\gamma_2^S - \gamma_1^S$  as a function of composition for the two simulated systems. The results for the differences  $\gamma_2^S - \gamma_1^S$  are displayed in the paper in Fig. 6.

Table S 1: Simulation results for systems with  $k_{12} = 1.35$  and  $\psi_\epsilon = 1.0$ . Quantities everywhere are given in reduced units. The reduced critical density is given by  $\rho_c^* = 0.304 = \frac{N\sigma_{11}^3}{V}$ .

| $x_1$ | $\frac{\rho^*}{2\rho_c^*}$ | $T^*$  | $p_1$ | $p_2$ | p     |
|-------|----------------------------|--------|-------|-------|-------|
| 0.10  | 1.0325                     | 2.0984 | 0.207 | 2.340 | 2.547 |
| 0.20  | 1.0186                     | 2.1951 | 0.449 | 2.010 | 2.549 |
| 0.30  | 1.0082                     | 2.2642 | 0.711 | 1.835 | 2.546 |
| 0.40  | 1.0021                     | 2.3056 | 0.988 | 1.556 | 2.545 |
| 0.50  | 1.0000                     | 2.3195 | 1.273 | 1.273 | 2.545 |

Table S 2: Simulations systems for  $k_{12} = 1.35$ ,  $\psi_\epsilon = 1.80$  Quantities everywhere are given in reduced units.

| $x_1$ | $\frac{\rho^*}{2\rho_c^*}$ | $T^*$  | $p_1$ | $p_2$ | p     |
|-------|----------------------------|--------|-------|-------|-------|
| 0.10  | 0.9592                     | 3.5414 | 0.354 | 3.103 | 3.457 |
| 0.20  | 0.9634                     | 3.4971 | 0.725 | 2.724 | 3.457 |
| 0.30  | 0.9736                     | 3.4204 | 1.114 | 2.353 | 3.467 |
| 0.40  | 0.9852                     | 3.3112 | 1.504 | 1.958 | 3.462 |
| 0.50  | 1.0000                     | 3.1695 | 1.888 | 1.562 | 3.449 |
| 0.60  | 1.0200                     | 2.9953 | 2.271 | 1.187 | 3.458 |
| 0.70  | 1.0450                     | 2.7887 | 2.643 | 0.821 | 3.464 |
| 0.80  | 1.0734                     | 2.5496 | 2.979 | 0.485 | 3.464 |
| 0.90  | 1.1069                     | 2.2780 | 3.249 | 0.202 | 3.452 |

Table S 3: Tabulated results for quantities relevant to generalized thermodynamic forces for simulations. with  $k_{12} = 1.35$  and  $\psi_\epsilon = 1.0$ . Results are obtained for different values of concentration  $x_1^{(0)}$  of component 1. Quantities everywhere are given in reduced units.

| $x_1$ | $L_1$  | $L_2$  | $L_2 - L_1$ |
|-------|--------|--------|-------------|
| 0.10  | 11.103 | 12.612 | 1.509       |
| 0.20  | 11.836 | 13.071 | 1.235       |
| 0.30  | 12.116 | 12.867 | 0.751       |
| 0.40  | 12.606 | 12.660 | 0.054       |
| 0.50  | 12.488 | 12.488 | 0.0         |

Table S 4: Tabulated results for quantities relevant to generalized thermodynamic forces for simulations. with  $k_{12} = 1.35$  and  $\psi_\epsilon = 1.80$ . Results are obtained for different values of concentration  $x_1$  of component 1. Quantities everywhere are given in reduced units.

| $x_1$ | $L_1$  | $L_2$  | $L_2 - L_1$ |
|-------|--------|--------|-------------|
| 0.10  | 16.152 | 17.264 | 0.707       |
| 0.20  | 16.743 | 16.876 | 0.133       |
| 0.30  | 17.458 | 16.432 | -1.026      |
| 0.40  | 17.689 | 16.508 | -1.181      |
| 0.50  | 18.473 | 16.435 | -2.038      |
| 0.60  | 18.231 | 15.170 | -3.112      |
| 0.70  | 18.463 | 15.477 | -2.986      |
| 0.80  | 18.403 | 14.063 | -4.340      |
| 0.90  | 18.152 | 13.065 | -5.087      |

Table S 5: Tabulated results for quantities relevant to generalized thermodynamic forces  $L_1^T$  with  $k_{12} = 1.35$  and  $\psi_\epsilon = 1.0$ . Results are obtained for different values of concentration  $x_1$  of component 1. Quantities everywhere are given in reduced units.

| $x_1$ | $L_1^T$ | $L_2^T$ | $L_2^T - L_1^T$ |
|-------|---------|---------|-----------------|
| 0.10  | 2.210   | 2.126   | -0.084          |
| 0.20  | 2.230   | 2.055   | -0.175          |
| 0.30  | 2.050   | 2.027   | -0.023          |
| 0.40  | 1.995   | 1.985   | -0.010          |
| 0.50  | 1.976   | 1.976   | 0.0             |

Table S 6: Tabulated results for quantities relevant to generalized thermodynamic forces  $L_1^T$  with  $k_{12} = 1.35$  and  $\psi_\epsilon = 1.80$ . Results are obtained for different values of concentration  $x_1$  of component 1. Quantities everywhere are given in reduced units.

| $x_1$ | $L_1^T$ | $L_2^T$ | $L_2^T - L_1^T$ |
|-------|---------|---------|-----------------|
| 0.10  | 1.800   | 1.850   | 0.050           |
| 0.20  | 1.780   | 1.839   | 0.059           |
| 0.30  | 1.840   | 1.899   | 0.059           |
| 0.40  | 1.878   | 1.955   | 0.078           |
| 0.50  | 1.996   | 1.964   | -0.032          |
| 0.60  | 1.990   | 2.105   | 0.115           |
| 0.70  | 2.153   | 2.257   | 0.104           |
| 0.80  | 2.285   | 2.255   | -0.030          |
| 0.90  | 2.508   | 2.660   | 0.152           |

Table S 7: Tabulated results for quantities relevant to generalized thermodynamic forces for simulations with  $k_{12} = 1.35$  and  $\psi_\epsilon = 1.0$ . Results are obtained for different values of concentration  $x_1^{(0)}$  of component 1. Quantities everywhere are given in reduced units.

| $x_1$ | $p_1$ | $p_2$ | $p$   | $\gamma_1^S$ | $\gamma_2^S$ | $\gamma_2^S - \gamma_1^S$ |
|-------|-------|-------|-------|--------------|--------------|---------------------------|
| 0.10  | 0.208 | 2.339 | 2.547 | 0.817        | 1.020        | 0.204                     |
| 0.20  | 0.459 | 2.102 | 2.561 | 0.896        | 1.026        | 0.130                     |
| 0.30  | 0.712 | 1.839 | 2.551 | 0.930        | 1.030        | 0.099                     |
| 0.40  | 0.987 | 1.554 | 2.541 | 0.971        | 1.019        | 0.048                     |
| 0.50  | 1.273 | 1.273 | 2.546 | 1.0          | 1.0          | 0.00                      |

Table S 8: Tabulated results for quantities relevant to generalized thermodynamic forces for simulations. with  $k_{12} = 1.35$  and  $\psi_\epsilon = 1.80$ . Results are obtained for different values of concentration  $x_1$  of component 1. Quantities everywhere are given in reduced units.

| $x_1$ | $p_1$ | $p_2$ | $p$   | $\gamma_1^S$ | $\gamma_2^S$ | $\gamma_2^S - \gamma_1^S$ |
|-------|-------|-------|-------|--------------|--------------|---------------------------|
| 0.10  | 0.354 | 3.103 | 3.457 | 1.024        | 0.997        | -0.027                    |
| 0.20  | 0.725 | 2.724 | 3.449 | 1.051        | 0.987        | -0.064                    |
| 0.30  | 1.114 | 2.353 | 3.467 | 1.071        | 0.970        | -0.102                    |
| 0.40  | 1.504 | 1.958 | 3.462 | 1.086        | 0.943        | -0.143                    |
| 0.50  | 1.888 | 1.562 | 3.450 | 1.094        | 0.906        | -0.189                    |
| 0.60  | 2.271 | 1.187 | 3.458 | 1.095        | 0.858        | -0.236                    |
| 0.70  | 2.643 | 0.821 | 3.464 | 1.090        | 0.790        | -0.300                    |
| 0.80  | 2.979 | 0.485 | 3.464 | 1.075        | 0.700        | -0.375                    |
| 0.90  | 3.249 | 0.202 | 3.451 | 1.046        | 0.585        | -0.461                    |
